# Supplementary material for: LLM+P: Empowering Large Language Models with Optimal Planning Proficiency
Source: arXiv:2304.11477 source file (2023-09-27)
Supplement: Supplementary file 1 [file appendix.tex]

\appendix
\section{Problem and Domain PDDL Files}
\label{sec:apx-pddl}
\begin{tcolorbox}[
    standard jigsaw,
    title=Problem PDDL Example,
    opacityback=0,
]
\PlanCode{(define (problem BW-rand-5)}\\
\PlanCode{\qquad(:domain blocksworld-4ops)}\\
\PlanCode{\qquad(:objects b1 b2 b3 b4 b5 )}\\
\PlanCode{\qquad(:init}\\
\PlanCode{\qquad\qquad(arm-empty)}\\
\PlanCode{\qquad\qquad(on b1 b2)}\\
\PlanCode{\qquad\qquad(on b2 b3)}\\
\PlanCode{\qquad\qquad(on b3 b5)}\\
\PlanCode{\qquad\qquad(on b4 b1)}\\
\PlanCode{\qquad\qquad(on-table b5)}\\
\PlanCode{\qquad\qquad(clear b4)}\\
\PlanCode{\qquad)}\\
\PlanCode{\qquad(:goal}\\
\PlanCode{\qquad\qquad(and}\\
\PlanCode{\qquad\qquad(on b1 b3)}\\
\PlanCode{\qquad\qquad(on b3 b5))}\\
\PlanCode{\qquad)}\\
\PlanCode{) }
\end{tcolorbox}

\begin{tcolorbox}[
    standard jigsaw,
    title=Domain PDDL Example,
    opacityback=0,
]
\PlanCode{(define (domain blocksworld-4ops)}\\
\PlanCode{\qquad  (:requirements :strips)}\\
\PlanCode{\qquad(:predicates (clear ?x)}\\
\PlanCode{\qquad\qquad             (on-table ?x)}\\
\PlanCode{ \qquad\qquad            (arm-empty)}\\
\PlanCode{\qquad\qquad             (holding ?x)}\\
\PlanCode{ \qquad\qquad            (on ?x ?y))}\\

\PlanCode{\qquad(:action pickup}\\
\PlanCode{\qquad\qquad  :parameters (?ob)}\\
\PlanCode{ \qquad\qquad :precondition (and (clear ?ob) (on-table ?ob) (arm-empty))}\\
\PlanCode{\qquad\qquad  :effect (and (holding ?ob) (not (clear ?ob)) }\\
\PlanCode{ \qquad\qquad\qquad   (not (on-table ?ob))           (not (arm-empty))))}\\

\PlanCode{\qquad(:action putdown}\\
\PlanCode{\qquad\qquad  :parameters  (?ob)}\\
\PlanCode{\qquad\qquad  :precondition (holding ?ob)}\\
\PlanCode{\qquad\qquad  :effect (and (clear ?ob) (arm-empty) (on-table ?ob) }\\
\PlanCode{\qquad\qquad\qquad (not (holding ?ob))))}\\

\PlanCode{\qquad(:action stack}\\
\PlanCode{\qquad\qquad  :parameters  (?ob ?underob)}\\
\PlanCode{\qquad\qquad  :precondition (and (clear ?underob) (holding ?ob))}\\
\PlanCode{\qquad\qquad  :effect (and (arm-empty) (clear ?ob) (on ?ob ?underob)}\\
\PlanCode{ \qquad\qquad\qquad              (not (clear ?underob)) (not (holding ?ob))))}\\

\PlanCode{\qquad(:action unstack}\\
\PlanCode{\qquad\qquad  :parameters  (?ob ?underob)}\\
\PlanCode{\qquad\qquad  :precondition (and (on ?ob ?underob) (clear ?ob) (arm-empty))}\\
\PlanCode{\qquad\qquad  :effect (and (holding ?ob) (clear ?underob) }\\
\PlanCode{ \qquad\qquad\qquad   (not (on ?ob ?underob)) (not (clear ?ob))}\\
\PlanCode{\qquad\qquad\qquad(not (arm-empty))))) }
\end{tcolorbox}
\section{Prompts for Different Methods}
\label{sec:apx-prompts}

\begin{tcolorbox}[
    standard jigsaw,
    title=The Prompt for \lmsp{} (no context),
    opacityback=0,
]

\promptdomain{}. Now consider a planning problem. The problem description is: \prompttask{}. Can you provide an optimal plan, in the way of a sequence of behaviors, to solve the problem?    
\end{tcolorbox}

\begin{tcolorbox}[
    standard jigsaw,
    title=The Prompt for \lmsp{} (with context),
    opacityback=0,
]
\promptdomain{}. An example planning problem is: \prompteg{}. A plan for the example problem is: \promptsol{}.
Now I have a new planning problem and its description is: \prompttask{}. 
Can you provide an optimal plan, in the way of a sequence of behaviors, to solve the problem?

\end{tcolorbox}
\begin{tcolorbox}[
    standard jigsaw,
    title=The Prompt for \lmp{} (no context),
    opacityback=0,
]
\promptdomain{}. Now consider a planning problem. The problem description is: \prompttask{}. Provide me with the problem PDDL file that describes the planning problem directly without further explanations.
\end{tcolorbox}

\begin{tcolorbox}[
    standard jigsaw,
    title=The Prompt for \lmp{} (with context),
    opacityback=0,
]
\promptdomain{}. An example planning problem is: \prompteg{}. The problem PDDL file to this problem is: \promptegpddl{}. Now I have a new planning problem and its description is: \prompttask{}. Provide me with the problem PDDL file that describes the planning problem directly without further explanations.   
\end{tcolorbox}
\newpage
\section{Example Failures}
\label{sec:apx-failures}
A list of representative failures for both the baseline methods and \lmsp{} is provided in this section.
\begin{tcolorbox}[
    standard jigsaw,
    title=Failure 1 of \lmsp{} (without context),
    opacityback=0,
]
\textbf{Problem (Barman):} \\\\
\PlanProblem{
You have 1 shaker with 3 levels, 4 shot glasses, 3 dispensers for 3 ingredients.
The shaker and shot glasses are clean, empty, and on the table.  \\\\
Your left and right hands are empty. The first ingredient of cocktail1 is ingredient1. The second ingredient of cocktail1 is ingredient3. The first ingredient of cocktail2 is ingredient2. The second ingredient of cocktail2 is ingredient3. The first ingredient of cocktail3 is ingredient1. The second ingredient of cocktail3 is ingredient2. \\\\
Your goal is to make 3 cocktails.
shot1 contains cocktail1. shot2 contains cocktail3. shot3 contains cocktail2.} \\\\
\textbf{GPT-3.5:} \\\\
1. Grasp the shaker with your left hand. \\
2. Grasp shot glass 1 with your right hand. \\
3. Fill shot glass 1 with ingredient 1 from the dispenser. \\
4. Pour ingredient 1 from shot glass 1 to the shaker. \\
5. Grasp shot glass 2 with your right hand. \\
6. Fill shot glass 2 with ingredient 2 from the dispenser. \\
7. Pour ingredient 2 from shot glass 2 to the shaker. \\
8. Grasp shot glass 3 with your right hand. \\
9. Fill shot glass 3 with ingredient 3 from the dispenser. \\
10. Pour ingredient 3 from shot glass 3 to the shaker. \\
11. Shake the shaker. \\
12. Pour the cocktail1 from the shaker to shot glass 1. \\
13. Empty shot glass 1. \\
14. Clean shot glass 1. \\
15. Pour the cocktail2 from the shaker to shot glass 2. \\
16. Empty shot glass 2. \\
17. Clean shot glass 2. \\
18. Pour the cocktail3 from the shaker to shot glass 3. \\
19. Empty shot glass 3. \\
20. Clean shot glass 3. \\
21. Leave the shaker on the table.
\end{tcolorbox}

\newpage

\begin{tcolorbox}[
    standard jigsaw,
    title=Failure 2 of \lmsp{} (without context),
    opacityback=0,
]
\textbf{Problem (BlocksWorld):} \\\\
\PlanProblem{
You have 3 blocks. 
b3 is on top of b2. 
b1 is on top of b3. 
b2 is on the table. 
b1 is clear. 
Your arm is empty. 
Your goal is to move the blocks. 
b2 should be on top of b3. 
b3 should be on top of b1.} \\\\
\textbf{GPT-3.5:} \\\\
Pickup b1 \\
Stack b1 on top of b2 \textbf{(Failed because b2 is not clear)} \\
Unstack b3 from b2 \\
Stack b3 on top of b1 \\
Putdown b1 
\end{tcolorbox}

\newpage

\begin{tcolorbox}[
    standard jigsaw,
    title=Failure 3 of \lmsp{} (without context),
    opacityback=0,
]
\label{apx:failure-grippers}
\textbf{Problem (Grippers):} \\\\
\PlanProblem{
There are 3 rooms and 2 balls. robot1 is in room1. robot4 is in room1. robot2 is in room1. robot3 is in room1. 
ball2 is in room3. ball1 is in room2. The robots' grippers are free. \\\\
Your goal is to transport the balls to their destinations. ball1 should be in room2. 
ball2 should be in room3.}  \\\\
\textbf{GPT-3.5:} \\\\
1. Robot1 picks up ball1 with its left gripper. \PlanComment{(Failed because robot1 and ball1 are in different rooms)} \\
2. Robot1 moves to room2. \\
3. Robot1 drops ball1 in room2. \\
4. Robot2 picks up ball2 with its right gripper. \\
5. Robot2 moves to room3. \\
6. Robot2 drops ball2 in room3.
\end{tcolorbox}

\newpage

\begin{tcolorbox}[
    standard jigsaw,
    title=Failure 1 of \lmsp{} (with in-context-learning),
    opacityback=0,
]
\textbf{Problem (Storage):} \\\\
\PlanProblem{
Depot storeareas are: depot48-1-1 depot48-1-2 depot48-2-1 depot48-2-2 \\
Container storeareas are: container-0-0 container-0-1 \\
Here is a map of depot storeareas: \\\\
depot48-1-1 depot48-1-2 \\
depot48-2-1 depot48-2-2 \\

According to the map, adjacent depot storeareas are connected.
All depot storeareas are in depot48. 
crate1 is on container-0-1. 
crate0 is on container-0-0. 
All crates and container storeareas are in container0. 
All container storeareas are connected to loadarea. 
depot48-2-1 and loadarea are connected. 
depot48-2-2 depot48-2-1 depot48-1-1 are clear. 
hoist0 is in depot48-1-2.
All hoists are available. \\\\
Your goal is to move all crates to depot48.}
\\\\
\textbf{GPT-3.5:} \\\\
Go out with hoist0 from depot48-1-2 to loadarea. \PlanComment{(Failed because depot48-1-2 and loadarea are not connected)} \\
Lift crate0 in container-0-0 in container 0 with hoist0 from loadarea. \\
Go in with hoist0 from loadarea to depot48-2-1. \\
Drop crate0 with hoist0 from depot48-2-1 to depot48-1-1 in depot48. \\
Go out with hoist0 from depot48-2-1 to loadarea. \\
Lift crate1 in container-0-1 in container 0 with hoist0 from loadarea. \\
Drop crate1 with hoist0 from loadarea to depot48-2-2 in depot48.
\end{tcolorbox}

\newpage

\begin{tcolorbox}[
    standard jigsaw,
    title=Failure 2 of \lmsp{} (with in-context-learning),
    opacityback=0,
]
\textbf{Problem (Termes):} \\\\
\PlanProblem{
The robot is on a grid with 4 rows and 3 columns. \\
pos-0-0 pos-0-1 pos-0-2 \\
pos-1-0 pos-1-1 pos-1-2 \\
pos-2-0 pos-2-1 pos-2-2 \\
pos-3-0 pos-3-1 pos-3-2 \\
The robot is at pos-2-0. 
The depot for new blocks is at pos-2-0. 
The maximum height of blocks is 3. \\\\
Your goal is to build blocks so that the height at pos-1-2 is 3. 
You cannot have an unplaced block at the end.}
\\\\
\textbf{GPT-3.5:} \\\\
Create block at pos-2-0 \\
move to pos-2-1 \\
place block at pos-1-2 \PlanComment{(Failed because pos-2-1 and pos-1-2 are not adjacent)} \\
move to pos-2-2 \\
place block at pos-1-2 \\
move to pos-2-1 \\
place block at pos-1-2 \\
move to pos-2-0 \\
place block at pos-1-2 \\
\end{tcolorbox}

\newpage

\begin{tcolorbox}[
    standard jigsaw,
    title=Failure 1 of  \lmp{} (without context),
    opacityback=0,
]
\textbf{Problem (Tyreworld):}  \\\\
\PlanProblem{
You have a jack, a pump, a wrench, a boot, 3 hubs, 3 nuts, 3 flat tyres, and 3 intact tyres. \\
The jack, pump, wrench, and intact tyres are in the boot.
The boot is unlocked but is closed. 
The intact tyres are not inflated. 
The flat tyres are on the hubs. 
The hubs are on the ground. 
The nuts are tight on the hubs. 
The hubs are fastened. \\\\
Your goal is to replace flat tyres with intact tyres on the hubs. Intact tyres should be inflated. The nuts should be tight on the hubs. The flat tyres, wrench, jack, and pump should be in the boot. The boot should be closed.} \\\\
\textbf{GPT-3.5:} \\
\\
\PlanCode{(define (problem replace-tyres)} \\
\PlanCode{\qquad (:domain tyre-replacement)} \\
\PlanCode{\qquad (:objects} \\
\PlanCode{\qquad \qquad jack pump wrench boot hub nut flat-tyre intact-tyre - object} \\
\PlanCode{\qquad  )} \\
\PlanCode{\qquad  (:init }\\
\PlanCode{\qquad\qquad    (in jack boot) }\\
\PlanCode{\qquad\qquad    (in pump boot) }\\
\PlanCode{\qquad\qquad    (in wrench boot) }\\
\PlanCode{\qquad\qquad   (in intact-tyre boot) }\\
\PlanCode{\qquad\qquad    (inflat intact-tyre) }\\
\PlanCode{\qquad\qquad    (on flat-tyre hub) }\\
\PlanCode{\qquad\qquad    (on-ground hub) }\\
\PlanCode{\qquad\qquad    (tight nut hub) }\\
\PlanCode{\qquad\qquad    (fasten hub) }\\
\PlanCode{\qquad\qquad    (closed boot) }\\
\PlanCode{\qquad  ) }\\
\PlanCode{\qquad  (:goal (and }\\
\PlanCode{\qquad\qquad    (not (on flat-tyre hub))} \\
\PlanCode{\qquad\qquad    (on intact-tyre hub) }\\
\PlanCode{\qquad\qquad    (inflat intact-tyre) }\\
\PlanCode{\qquad\qquad    (tight nut hub) }\\
\PlanCode{\qquad\qquad    (in jack boot) }\\
\PlanCode{\qquad\qquad    (in pump boot) }\\
\PlanCode{\qquad\qquad    (in wrench boot) }\\
\PlanCode{\qquad\qquad    (in intact-tyre boot) }\\
\PlanCode{\qquad\qquad    (closed boot) }\\
\PlanCode{\qquad  )) }\\
\PlanCode{) }
\end{tcolorbox}
